# Supplementary material for: High-speed Tracking with Multi-kernel Correlation Filters
Source: arXiv:1806.06418 source file (2018-06-17)
Supplement: Supplementary file 2 [file hspeedMKCF__Supp_CVPR18_.pdf]

## Supplementary Material

### High-speed Tracking with Multi-kernel Correlation Filters

Ming Tang<sup>1,2</sup>, Bin Yu<sup>1,2</sup>, Fan Zhang<sup>3</sup>, and Jinqiao Wang<sup>1,2</sup>

<sup>1</sup>University of Chinese Academy of Sciences, Beijing, China

<sup>2</sup>National Lab of Pattern Recognition, Institute of Automation, CAS, Beijing 100190, China

<sup>3</sup>School of Info. & Comm. Eng., Beijing University of Posts and Telecommunications

#### Abstract

*This supplementary material includes 1) the experimental results on OTB2015, 2) the proof of Theorem 1.*

#### 1. Experimental Results on OTB2015

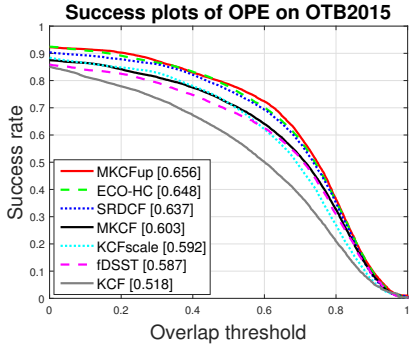

Figure 1. The success plot of MKCFup, KCF, KCFscale, MKCF, SRDCF, fDSST, and ECO\_HC on small move sequences of OTB2015. The AUCs of the trackers on the sequences are reported in the legends.

#### 2. Proof of Upper Bound of MKCF Objective Function [2]

**Lemma 1** Suppose  $\mathbf{a}_m$  is a vector,  $m = 1, \dots, M$ . Then,

$$\left\| \sum_{m=1}^M \mathbf{a}_m \right\|_2^2 \leq (2M + 1) \sum_{m=1}^M \|\mathbf{a}_m\|_2^2.$$

The equality holds when  $\mathbf{a}_m = \mathbf{a}_n$ , where  $m = 1, \dots, M$  and  $n = 1, \dots, M$ .

Proof of Lemma 1:

It is true that

$$\begin{aligned} \left\| \sum_{m=1}^M \mathbf{a}_m \right\|_2^2 &= \left( \sum_{m=1}^M \mathbf{a}_m \right)^\top \left( \sum_{m=1}^M \mathbf{a}_m \right) = \\ &= \sum_{m=1}^M \mathbf{a}_m^\top \sum_{m=1}^M \mathbf{a}_m = \sum_{m=1}^M \mathbf{a}_m^\top \mathbf{a}_m + 2 \sum_{m=1}^M \sum_{n=1}^M \mathbf{a}_m^\top \mathbf{a}_n. \end{aligned}$$

It is also true that

$$\begin{aligned} \mathbf{a}_m^\top \mathbf{a}_m + \mathbf{a}_n^\top \mathbf{a}_n - 2\mathbf{a}_m^\top \mathbf{a}_n &= \\ \mathbf{a}_m^\top (\mathbf{a}_m - \mathbf{a}_n) - \mathbf{a}_n^\top (\mathbf{a}_m - \mathbf{a}_n) &= \\ (\mathbf{a}_m - \mathbf{a}_n)^\top (\mathbf{a}_m - \mathbf{a}_n) &= \|\mathbf{a}_m - \mathbf{a}_n\|_2^2 \geq 0. \end{aligned}$$

Therefore,

$$\begin{aligned} \mathbf{a}_m^\top \mathbf{a}_m + \mathbf{a}_n^\top \mathbf{a}_n &\geq 2\mathbf{a}_m^\top \mathbf{a}_n, \\ \sum_{m=1}^M \mathbf{a}_m^\top \mathbf{a}_m + M\mathbf{a}_n^\top \mathbf{a}_n &\geq 2 \sum_{m=1}^M \mathbf{a}_m^\top \mathbf{a}_n, \\ M \sum_{m=1}^M \mathbf{a}_m^\top \mathbf{a}_m + M \sum_{n=1}^M \mathbf{a}_n^\top \mathbf{a}_n &\geq 2 \sum_{n=1}^M \sum_{m=1}^M \mathbf{a}_m^\top \mathbf{a}_n, \\ 2M \sum_{m=1}^M \mathbf{a}_m^\top \mathbf{a}_m &\geq 2 \sum_{m=1}^M \sum_{n=1}^M \mathbf{a}_m^\top \mathbf{a}_n. \end{aligned}$$

Therefore,

$$\begin{aligned} \left\| \sum_{m=1}^M \mathbf{a}_m \right\|_2^2 &= \sum_{m=1}^M \mathbf{a}_m^\top \mathbf{a}_m + 2 \sum_{m=1}^M \sum_{n=1}^M \mathbf{a}_m^\top \mathbf{a}_n \\ &\leq \sum_{m=1}^M \mathbf{a}_m^\top \mathbf{a}_m + 2M \sum_{m=1}^M \mathbf{a}_m^\top \mathbf{a}_m \\ &= (2M + 1) \sum_{m=1}^M \mathbf{a}_m^\top \mathbf{a}_m. \end{aligned}$$

That is,

$$\left\| \sum_{m=1}^M \mathbf{a}_m \right\|_2^2 \leq (2M+1) \sum_{m=1}^M \|\mathbf{a}_m\|_2^2.$$

It is clear that the equality holds when  $\mathbf{a}_m = \mathbf{a}_n$ , where  $m = 1, \dots, M$  and  $n = 1, \dots, M$ .

Q.E.D.

### 2.1. Proof of Upper Bound

According to Lemma 1,

$$\left\| \mathbf{y} - \sum_{m=1}^M d_m \mathbf{K}_m \boldsymbol{\alpha} \right\|_2^2 \leq (2M+1) \sum_{m=1}^M \|\mathbf{y}_c - d_m \mathbf{K}_m \boldsymbol{\alpha}\|_2^2.$$

Therefore,  $U_{F(\boldsymbol{\alpha}, \mathbf{d})}$  is the upper bound of  $F(\boldsymbol{\alpha}, \mathbf{d})$ , and the upper bound is reached when  $d_m \mathbf{K}_m \boldsymbol{\alpha} = d_n \mathbf{K}_n \boldsymbol{\alpha}$ , where  $m = 1, \dots, M$  and  $n = 1, \dots, M$ .

Q.E.D.

### 3. Proof of Theorem 1

In the extension of MKCF with upper bound, to optimize the unconstrained problem

$$\min_{\boldsymbol{\alpha}_p, \mathbf{d}_p} F_p(\boldsymbol{\alpha}_p, \mathbf{d}_p), \quad (1)$$

we achieve that

$$\boldsymbol{\alpha}_p = \left( \sum_{j=1}^p \sum_{m=1}^M \beta_m^j ((d_{m,p} \mathbf{K}_m^j)^2 + \lambda d_{m,p} \mathbf{K}_m^j) \right)^{-1} \cdot \sum_{j=1}^p \sum_{m=1}^M \beta_m^j d_{m,p} \mathbf{K}_m^j \mathbf{y}_c, \quad (2)$$

and

$$d_{m,p} = \frac{d_{m,p}^N}{d_{m,p}^D}, \quad (3)$$

where

$$\begin{aligned} d_{m,p}^N &= (1 - \gamma_m) d_{m,p-1}^N + \gamma_m (\mathbf{K}_m^p \boldsymbol{\alpha}_p)^\top (2\mathbf{y}_c - \lambda \boldsymbol{\alpha}_p), \\ d_{m,p}^D &= (1 - \gamma_m) d_{m,p-1}^D + 2\gamma_m (\mathbf{K}_m^p \boldsymbol{\alpha}_p)^\top (\mathbf{K}_m^p \boldsymbol{\alpha}_p), \end{aligned}$$

when  $p > 1$ . If  $p = 1$ , then

$$\begin{aligned} d_{m,1}^N &= (\mathbf{K}_m^1 \boldsymbol{\alpha}_1)^\top (2\mathbf{y}_c - \lambda \boldsymbol{\alpha}_1), \\ d_{m,1}^D &= (\mathbf{K}_m^1 \boldsymbol{\alpha}_1)^\top (\mathbf{K}_m^1 \boldsymbol{\alpha}_1). \end{aligned}$$

To simplify the denotation, in the proof,  $d_{m,p}$  expresses the kernel weight  $d_{m,p}^t$  of the  $t^{\text{th}}$  iteration of  $\boldsymbol{\alpha}_p$  and  $\mathbf{d}_p$ .

### 3.1. Proof of First Conclusion

According to Eq. (2), we set  $\boldsymbol{\alpha}_p = \mathbf{D}_p^{-1} \mathbf{N}_p \mathbf{y}_c$ , where

$$\mathbf{D}_p = \sum_{j=1}^p \sum_{m=1}^M \beta_m^j ((d_{m,p} \mathbf{K}_m^j)^2 + \lambda d_{m,p} \mathbf{K}_m^j)$$

and

$$\mathbf{N}_p = \sum_{j=1}^p \sum_{m=1}^M \beta_m^j d_{m,p} \mathbf{K}_m^j.$$

It is clear that both  $\mathbf{D}_p$  and  $\mathbf{N}_p$  are positive definite because  $\beta_m^j > 0$ ,  $d_{m,p} > 0$ ,  $\lambda > 0$ , and  $\mathbf{K}_m^j$  is positive definite. Because  $\mathbf{K}_m^j$  is circulant Gram matrix, we have  $\mathbf{K}_m^j = \mathbf{U} \boldsymbol{\Sigma}_m^j \mathbf{U}^H$ , where  $\mathbf{U} = \frac{1}{\sqrt{l}} \mathbf{F}_l^{-1}$  and  $\mathbf{F}_l$  is the 1-D discrete Fourier transform matrix [1]. Because the linear combination of circulant matrices is also circulant, we have

$$\mathbf{D}_p = \mathbf{U} \left( \sum_{j=1}^p \sum_{m=1}^M \beta_m^j (d_{m,p}^2 (\boldsymbol{\Sigma}_m^j)^2 + \lambda d_{m,p} \boldsymbol{\Sigma}_m^j) \right) \mathbf{U}^H$$

and

$$\mathbf{N}_p = \mathbf{U} \left( \sum_{j=1}^p \sum_{m=1}^M \beta_m^j d_{m,p} \boldsymbol{\Sigma}_m^j \right) \mathbf{U}^H.$$

Let  $\boldsymbol{\Sigma}_m^j = \text{diag}(\sigma_{m,1}^j, \dots, \sigma_{m,l}^j)$ ,  $\sigma_{m,n}^j > 0$ ,  $n = 1, \dots, l$ . Then the  $n^{\text{th}}$  eigenvalue of  $\mathbf{D}_p^{-1} \mathbf{N}_p$  is

$$\begin{aligned} \sigma_{\boldsymbol{\alpha}_p, n} &\equiv \frac{\sum_{j=1}^p \sum_{m=1}^M \beta_m^j d_{m,p} \sigma_{m,n}^j}{\sum_{j=1}^p \sum_{m=1}^M \beta_m^j d_{m,p} \sigma_{m,n}^j (d_{m,p} \sigma_{m,n}^j + \lambda)} \\ &= (\lambda + b_n)^{-1}, \end{aligned}$$

where

$$b_n = \frac{\sum_{j=1}^p \sum_{m=1}^M \beta_m^j d_{m,p}^2 (\sigma_{m,n}^j)^2}{\sum_{j=1}^p \sum_{m=1}^M \beta_m^j d_{m,p} \sigma_{m,n}^j}.$$

It is clear that  $b_n > 0$ .

According to Eq. (3), we also have

$$\begin{aligned} d_{m,p}^N &= \sum_{j=1}^p \beta_m^j (\mathbf{K}_m^j \boldsymbol{\alpha}_p)^\top (2\mathbf{y}_c - \lambda \boldsymbol{\alpha}_p) \\ &= \mathbf{y}_c^\top \sum_{j=1}^p \beta_m^j \mathbf{N}_p \mathbf{D}_p^{-1} \mathbf{K}_m^j (2\mathbf{I} - \lambda \mathbf{D}_p^{-1} \mathbf{N}_p) \mathbf{y}_c \\ &= \mathbf{y}_c^\top \mathbf{D}_{m,p}^N \mathbf{y}_c, \end{aligned}$$

where  $\mathbf{D}_{m,p}^N = \mathbf{N}_p \mathbf{D}_p^{-1} \sum_{j=1}^p \beta_m^j \mathbf{K}_m^j (2\mathbf{I} - \lambda \mathbf{D}_p^{-1} \mathbf{N}_p)$ , and its  $n^{\text{th}}$  eigenvalue is

$$\sigma_{m,p,n}^N = \sigma_{\boldsymbol{\alpha}_p, n} (2 - \lambda \sigma_{\boldsymbol{\alpha}_p, n}) \sum_{j=1}^p \beta_m^j \sigma_{m,n}^j.$$

$\because \lambda \sigma_{\alpha_p, n} = \lambda(\lambda + b_n)^{-1} < 1, \therefore 2 - \lambda \sigma_{\alpha_p, n} > 1, \therefore \sigma_{m, p, n}^N > 0, n = 1, \dots, l, \therefore \mathbf{D}_{m, p}^N$  is positive definite, and  $d_{m, p}^N > 0$ . It is obvious that  $d_{m, p}^D > 0$ . Consequently,

$$d_{m, p}^{t+1} = \frac{d_{m, p}^N}{d_{m, p}^D} > 0,$$

where  $m = 1, \dots, M$ .

Q.E.D.

### 3.2. Proof of Second Conclusion

According to Eq. (2), we have

$$\begin{aligned} d_{m, p}^D &= 2 \sum_{j=1}^p \beta_m^j (\mathbf{K}_m^j \alpha_p)^\top (\mathbf{K}_m^j \alpha_p) \\ &= \mathbf{y}_c^\top 2 \sum_{j=1}^p \beta_m^j \mathbf{N}_p \mathbf{D}_p^{-1} (\mathbf{K}_m^j)^2 \mathbf{D}_p^{-1} \mathbf{N}_p \mathbf{y}_c \\ &= \mathbf{y}_c^\top \mathbf{D}_{m, p}^D \mathbf{y}_c \end{aligned}$$

where  $\mathbf{D}_{m, p}^D = 2 \mathbf{N}_p \mathbf{D}_p^{-1} \sum_{j=1}^p \beta_m^j (\mathbf{K}_m^j)^2 \mathbf{D}_p^{-1} \mathbf{N}_p$ , and its  $n^{\text{th}}$  eigenvalue is

$$\sigma_{m, p, n}^D = 2 \sigma_{\alpha_p, n}^2 \sum_{j=1}^p \beta_m^j (\sigma_{m, n}^j)^2.$$

Then, according to Eq. (3),

$$d_{m, p}^{t+1} = \frac{d_{m, p}^N}{d_{m, p}^D} = \frac{\mathbf{y}_c^\top \mathbf{D}_{m, p}^N \mathbf{y}_c}{\mathbf{y}_c^\top \mathbf{D}_{m, p}^D \mathbf{y}_c} = \frac{\mathbf{y}_c^\top \mathbf{U} \Sigma_{m, p}^N \mathbf{U}^H \mathbf{y}_c}{\mathbf{y}_c^\top \mathbf{U} \Sigma_{m, p}^D \mathbf{U}^H \mathbf{y}_c}.$$

Let  $\mathbf{U}^H \mathbf{y}_c = (y_{u, 1}, \dots, y_{u, l})$ ,  $c_n^N = \sum_{j=1}^p \beta_m^j \sigma_{m, n}^j$ , and  $c_n^D = \sum_{j=1}^p \beta_m^j (\sigma_{m, n}^j)^2$ . Then

$$d_{m, p}^{t+1} = \frac{\sum_{n=1}^l y_{u, n}^2 c_n^N \sigma_{\alpha_p, n} (2 - \lambda \sigma_{\alpha_p, n})}{2 \sum_{n=1}^l y_{u, n}^2 c_n^D \sigma_{\alpha_p, n}^2}.$$

Let  $c_{\max}^N = \max_n c_n^N$ ,  $c_{\min}^N = \min_n c_n^N$ ,  $c_{\max}^D = \max_n c_n^D$ ,  $c_{\min}^D = \min_n c_n^D$ ,  $y_{\max} = \max_n y_{u, n}$ ,  $y_{\min} = \min_n y_{u, n}$ ,

$$c_l = \frac{y_{\min}^2 c_{\min}^N}{y_{\max}^2 c_{\max}^N}, \quad c_u = \frac{y_{\max}^2 c_{\max}^N}{y_{\min}^2 c_{\min}^N},$$

and

$$\sigma_r = \frac{\sum_{n=1}^l \sigma_{\alpha_p, n} (2 - \lambda \sigma_{\alpha_p, n})}{2 \sum_{n=1}^l \sigma_{\alpha_p, n}^2}.$$

Then

$$c_l \cdot \sigma_r < d_{m, p}^{t+1} < c_u \cdot \sigma_r.$$

Furthermore,

$$\begin{aligned} \sigma_r &= \frac{\sum_{n=1}^l (\lambda + b_n)^{-1} (2(\lambda + b_n) - \lambda) (\lambda + b_n)^{-1}}{2 \sum_{n=1}^l (\lambda + b_n)^{-2}} \\ &= \frac{\sum_{n=1}^l (\lambda + b_n)^{-2} (\lambda + 2b_n)}{2 \sum_{n=1}^l (\lambda + b_n)^{-2}} \\ &= \frac{1}{2} \lambda + \frac{\sum_{n=1}^l b_n (\lambda + b_n)^{-2}}{\sum_{n=1}^l (\lambda + b_n)^{-2}}. \end{aligned}$$

Let  $\sigma_{m, \max}^j = \max_n \sigma_{m, n}^j$ ,  $\sigma_{m, \min} = \min_n \sigma_{m, n}^j$ ,

$$\begin{aligned} b_{\max} &= \frac{\sum_{j=1}^p \sum_{m=1}^M \beta_m^j d_{m, p}^2 (\sigma_{m, \max}^j)^2}{\sum_{j=1}^p \sum_{m=1}^M \beta_m^j d_{m, p} \sigma_{m, \min}^j}, \\ b_{\min} &= \frac{\sum_{j=1}^p \sum_{m=1}^M \beta_m^j d_{m, p}^2 (\sigma_{m, \min}^j)^2}{\sum_{j=1}^p \sum_{m=1}^M \beta_m^j d_{m, p} \sigma_{m, \max}^j}. \end{aligned}$$

Then,  $b^{\min} \leq b_n \leq b^{\max}$ , and

$$\frac{1}{2} \lambda + b^{\min} \leq \sigma_r \leq \frac{1}{2} \lambda + b^{\max},$$

$$\frac{c_l}{2} \lambda + c_l \cdot b^{\min} < d_{m, p}^{t+1} < \frac{c_u}{2} \lambda + c_u \cdot b^{\max}.$$

where  $m = 1, \dots, M$ .

Q.E.D.

## References

- [1] P. David. *Circulant Matrices*. Chelsea Publishing Company, 2<sup>nd</sup> edition, 1994. [2](#)
- [2] M. Tang and J. Feng. Multi-kernel correlation filter for visual tracking. In *Proc. International Conference on Computer Vision*, 2015. [1](#)
